# Supplementary material for: FreshGNN: Reducing Memory Access via Stable Historical Embeddings for Graph Neural Network Training
Source: arXiv:2301.07482 source file (2024-03-24)
Supplement: Supplementary file 1 [file appendix.tex]

% \section{Experimental Details}
% lr, dropout, weight-decay

\section{Comparison of \system Trainig Curves}
\begin{figure}[h]
    \centering
    \begin{subfigure}[b]{0.4\textwidth}
        \centering
		\includegraphics
		[width=\textwidth]{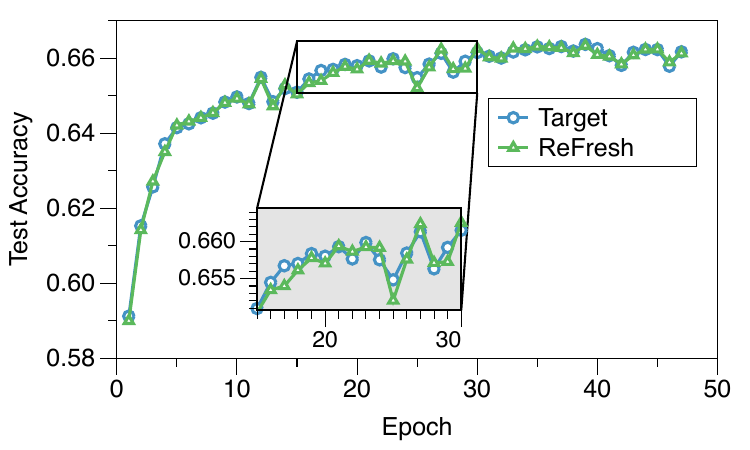}
	    \caption{SAGE}
    \end{subfigure}
     % \hfill
    \begin{subfigure}[b]{0.4\textwidth}
        \centering
		\includegraphics
		[width=\textwidth]{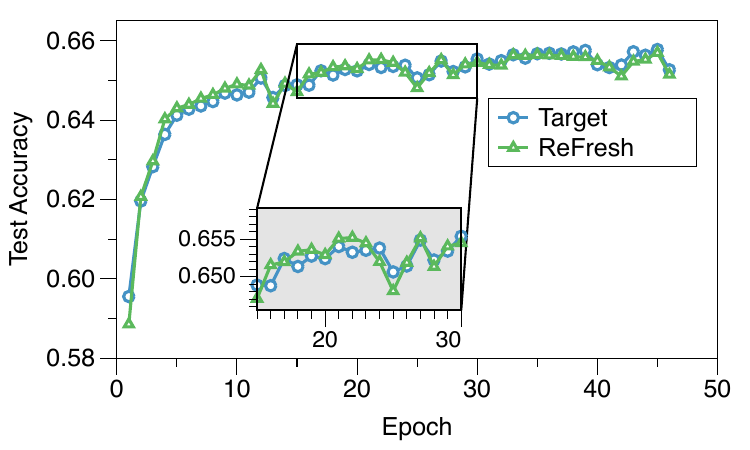}
		\caption{GCN}
    \end{subfigure}
    \caption{Test accuracy curve for \system and target neighbor sampling with same mini-batches and initial parameters on \texttt{ogbn-papers100M}.}
\end{figure}

{In this experiment, we compare the test accuracy after each epoch in the training process of \system and the target neighbor sampling on \texttt{ogbn-papers100M}. The weight of the two counterparts are initialized as the same, and for each iteration, the sampled mini-batch is the same. For both GraphSAGE and GCN model, the curves are aligned quite well, showing that using the historical embedding cache has little change on the update of parameters.}
